# Supplementary material for: Causal Discovery over High-Dimensional Structured Hypothesis Spaces with Causal Graph Partitioning
Source: arXiv:2406.06348 source file (2025-03-03)
Supplement: Supplementary file 1 [file appendix-ecoli.tex]

\begin{figure}[h]
    \centering
    \includegraphics[width=0.5\linewidth]{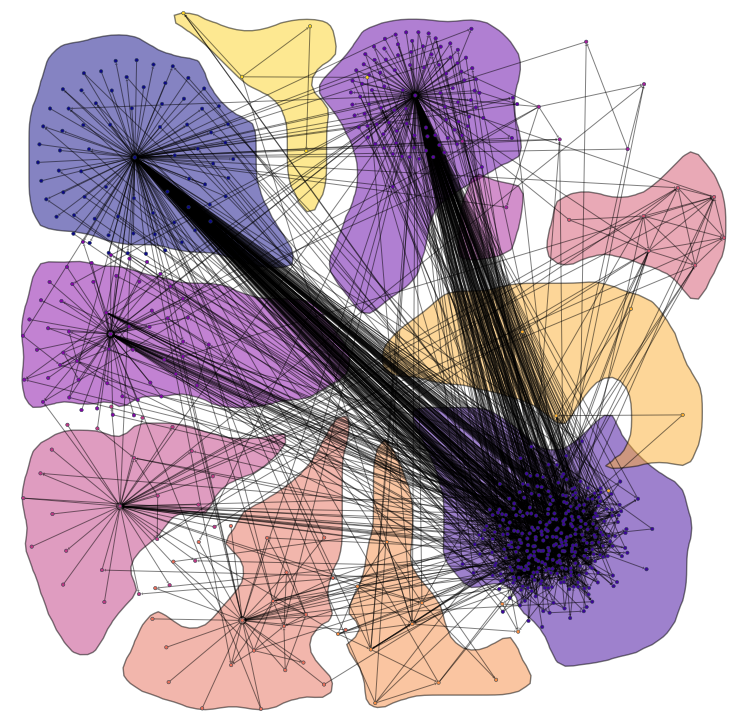}
    \caption{Top 5 hubs of synthetically tuned E.coli network with the proximity-based model and Girvan-Newman partition. }
\label{fig:ecoli}
\end{figure}
