# Supplementary material for: Causal Discovery over High-Dimensional Structured Hypothesis Spaces with Causal Graph Partitioning
Source: arXiv:2406.06348 source file (2025-03-03)
Supplement: Supplementary file 2 [file appendix-justification-GES.tex]

In our empirical study, we use Greedy Equivalence Search (GES) for  $\mathscr{A}$. This algorithm assumes causal sufficiency, however, in our proof we assume that $\mathscr{A}$ allows for latent confounders. Algorithms that allow for latent confounders include FCI, RCD and DCD. We rule out FCI because only estimates the equivalence class of ADMGs. We rule out RCD because it assumes a non-Gaussian setting. In the future, we wish to incorporate the DCD algorithm in our empirical evaluation. By using GES, it is unclear if $\mathscr{A}(X_{S}) = L(G^*, S)$ as in Assumption \ref{assume:consistent_learner}. The empirical results of the expansive causal partition using GES suggest that Algorithm \ref{alg:screening_finite} effectively screens extraneous edges from the graph. This may mean that GES also infers projected edges, although an additional study is needed to understand this. Moreover, an attractive aspect of GES is the natural extension to GIES \cite{hauser2015jointly} which jointly learns from observational and interventional data.
