# Supplementary material for: Causal Discovery over High-Dimensional Structured Hypothesis Spaces with Causal Graph Partitioning
Source: arXiv:2406.06348 source file (2025-03-03)
Supplement: Supplementary file 3 [file appendix-metrics.tex]

\begin{itemize}
    \item SHD
    \item TPR
    \item FPR
\end{itemize}
