# Supplementary material for: Causal Discovery over High-Dimensional Structured Hypothesis Spaces with Causal Graph Partitioning
Source: arXiv:2406.06348 source file (2025-03-03)
Supplement: Supplementary file 4 [file OLD_appendix-deferred_proofs.tex]

\begin{proof}[{\bf Proof of Lemma~\ref{lemma:superstructure}}]
    Because the superstructure $G$ is a superset of $G^*$, $(x,y) \in G^*$ or $(y,x) \in G^* \Rightarrow \exists$ some (un)directed edge in $G$. Because $\{S_1, ..., S_N\}$ is edge covering $\exists S_j$ such that $x,y \in S_j$. Since $\mathscr{A}(X_{S_j}) = L(G^*, S_j)$, $(x,y) \in G^* \Rightarrow (x,y) \in \mathscr{A}(X_{S_j})$ and the same for $(y,x)$. Therefore $(x,y) \notin \mathscr{A}(X_{S_j}) \Rightarrow (x,y) \notin G^*$.
\end{proof}

\begin{lemma}[Conflict $\Rightarrow$ projected edge]
\label{lemma:conflict_to_projected}

If a conflict occurs on nodes $u,v \in S_i\cap S_j$, then any edges $(u,v), (v,u), \{u,v\}$ in $\mathscr{A}(X_{S_i})$ and $\mathscr{A}(X_{S_j})$ are projected. 
 \end{lemma}

\begin{proof}[{\bf Proof of Lemma~\ref{lemma:conflict_to_projected}}]
    For all $i$, any edge in $\mathscr{A}(X_{S_i})$ is either in $G^*$ or projected. From Assumption \ref{assume:consistent_learner}, $(u,v) \in G^* \Rightarrow (u,v) \in\mathscr{A}(X_{S_i})$ for all subsets $S_i \ni u,v$. This implies that after union all $\mathscr{A}(X_{S_i})$ are in agreement for edges in $G^*$, and therefore a conflict only arises for projected edges. 
\end{proof}

\begin{proof}[{\bf Proof of Lemma~\ref{lemma:projected_to_conflict}}]
    By Assumption~\ref{assume:consistent_learner}, if $(u,v)\in\mathscr{A}(X_{S_i})$ is a directed projected edge then $G^*$ contains a directed path from $u$ to $v$. Because $G$ is a perfect superstructure of $G^*$, $G$ must therefore contain a potentially directed path from $u$ to $v$. If $(u,v)\not\in G$, then the statement of the lemma is satisfied. If $(u,v)\in G$, then because $G$ contains a potentially directed path from $u$ to $v$ Defn. \ref{def:causal_partition} implies that there exists an $S_j$ s.t. $u,v \in S_j$ and a vertex $x \in S_j$, where $x$ is an intermediate along the potentially directed path $P(u,v)$. In particular, Defn. \ref{def:ladmg} implies that $(u,v)\notin \mathscr{A}(X_{S_j})$ because all intermediates along $P(u,v)$ are not unobserved in $S_j$. This implies $\mathscr{A}(X_{S_i})$ and $\mathscr{A}(X_{S_j})$ are not in agreement over $(u,v)$.    
\end{proof}


\begin{proof}[{\bf Proof of Lemma~\ref{lem:causal-expansion}}]
    We first establish that $\{S'_1,\dots,S'_N\}$ is edge-covering with respect to $G$. Given the initial partition $\{S_1,\dots,S_N\}$ is vertex-covering, $\forall u\in V$ $\exists i\in [N]$ such that $u\in S_i$. For such $S_i$, it holds that $\forall v\in V$ such that $u\sim_{G} v$, either $v\in S_i$ or $v\in \outerboundary(S_i)$. In the both cases, the edge from $u$ to $v$ is thus covered by $S'_i$.

    We now establish the second property. Consider $u,v\in S'_i$ such that $(u,v) \in G$ and $G$ contains a potentially directed path $(u,x_1,\dots,x_k,v)$ such that $x_p\not\in S'_i$ for all $p \in [k]$. First, observe that the fact $x_1\not\in S'_i$ and $u\sim_{G} x_1$ implies that $u\in \outerboundary(S_i)\setminus S_i$, as if $u$ were i  $S_i$ then $x_1$ would be in $S'_i$. Because the original partition is vertex-covering, this implies $\exists j\neq i$ such that $u\in S_j \subseteq S'_j$. Moreover, $u\sim_{G} x_1$ and $u\sim_{G} v$, which implies $x_1, v \in \outerboundary(S_j) \cup S_j$. Thus by construction $\{x_1, v, u\}\subseteq S'_j$ for $j\neq i$, thus establishing the second property.
\end{proof}


\begin{proof}[\bf Proof of Theorem~\ref{thm:merge_operation}]
Assumption~\ref{assume:consistent_learner} implies that in the infinite data limit $\mathscr{A}(X_{S_i}) = L(G^*_M, S_i)$ for all $i\in[N]$. In particular Lemma~\ref{lemma:superstructure} and the fact that $G$ is a perfect superstructure of $G^*$, and thus a perfect superstructure of $G^*_M$, imply that the edges of $\mathscr{A}(X_{S_i})$, denoted $E_i$, can be expressed as a disjoint union: $E_i = E^*_i \sqcup P_i$, where $E^*_i$ is the set of all directed edges between nodes in $S_i$ which exist in $G^*_M$, and $P_i$ is the set of projected edges. Because $\{S_1,\dots,S_N\}$ is a causal partition, it is edge-covering with respect to $G$. Moreover by assumption $G$ is a perfect superstructure, so $\{S_1,\dots,S_N\}$ is therefore also edge covering with respect to $G^*_M$. Thus $\cup_i E^*_i$ contains all edges in $G^*_M$. Thus in order to show that \screenprojections\ recovers $G^*_M$, we want to show that for all $i = 1,\dots,N$, \screenprojections\ adds exactly the edges in $E^*_i$ to the output edge set $E^*$.

By Assumption~\ref{assume:consistent_learner}, the projected edges in $P_i$ are of two varieties: bi-directed projected edges $B(P_i)$ and directed projected edges $D(P_i)$. By Lemma~\ref{lemma:superstructure}, all bidirected edges in $\mathscr{A}(X_{S_i})$ are elements of $B(P_i)$. Thus in Line~\ref{line:discard_bidirected_and_not_in_ss} of  Algorithm~\ref{alg:screening}, discarding all bi-directed edges from the output discards all elements of $B(P_i)$. Thus no elements of $B(P_i)$ will be added to $E^*$.

We now consider directed projected edges. Because $\{S_1,\dots,S_N\}$ is a causal partition, Lemma~\ref{lemma:projected_to_conflict} implies that for any projected directed edge $(u,v) \in D(P_i)$, either $(u,v)$ is not in the superstructure $G$ or there exists $p \neq j$ such that $u,v \in S_p$ and $(u,v)\not\in\mathscr{A}(X_{S_p})$. In the first case, if $(u,v)$ is not in superstructure $G$ then it will be discarded in Line~\ref{line:discard_bidirected_and_not_in_ss} of Algorithm~\ref{alg:screening}, and thus will not be added to $E^*$. In the second case, exists $p \neq j$ such that $u,v \in S_p$ and $(u,v)\not\in\mathscr{A}(X_{S_p})$, so in Line~\ref{line:favor_no_edge}, $(u,v)$ will not be added to $E^*$. Thus no projected directed edge will be added to $E^*$.

We have thus shown that the procedure \screenprojections\ defined in Algorithm~\ref{alg:screening} does not add any edges from $P_i$ to the output edge set $E^*$. It remains to show that \screenprojections\ does add all edges in $E^*_i$ to $E^*$ for every subset $i = 1,\dots,N$. By Assumption~\ref{assume:consistent_learner} in the infinite data limit $(u,v) \in \mathscr{A}(X_{S_i})$ for all $S_i \ni u, v$ for any $(u,v) \in G^*_M$. Because $G$ is a perfect superstructure, Line~\ref{line:discard_bidirected_and_not_in_ss} will ensure that $E_i \supseteq E^*_i$. Moreover, in the infinite data limit for all $(u,v) \in E_i^*$, $(u,v)\in \mathscr{A}(X_{S_i}) \ \forall S_i \ni u,v$. Thus in the infinite data limit Line~\ref{line:favor_no_edge}  adds all elements of $E^*_i$, and so the output edge set $E^*$ is exactly equal to the set of edges on $G^*_M$.
\end{proof}
